# Supplementary material for: Software Testing for Extended Reality Applications: A Systematic Mapping Study
Source: arXiv:2501.08909 source file (2025-03-20)
Supplement: Supplementary file 1 [file appendix_B.tex]

\newgeometry{left=2cm, right=2cm}

\section{Publication venues of the primary studies} \label{appendix:venue}

\begingroup
\DefTblrTemplate{firsthead, middlehead,lasthead}{default}{} % <---
\DefTblrTemplate{contfoot-text}{normal}{\scriptsize\textit{Continued on the next page}}
\SetTblrTemplate{contfoot-text}{normal}

\begin{longtblr}{ colspec = {cXllc}, rowhead=1} 
\# & Venue & Type & Domain & No. \\ \hline
1 & International Symposium on Software Testing and Analysis (ISSTA) & Symposium & SWE & 2 \\
2 & Symposium on Virtual Reality (SVR) & Symposium & XR & 2 \\
3 & Software Testing, Verification and Reliability (STVR) & Journal & SWE & 2 \\
4 & International Workshop on Virtual and Augmented Reality Software Engineering (VARSE) & Workshop & XR + SWE & 2 \\
5 & International Conference on Automated Software Engineering (ASE) & Conference & SWE & 2 \\
6 & ACM Symposium on Virtual Reality Software and Technology & Symposium & XR & 1 \\
7 & International Conference on Vocational Education and Training (ICOVET) & Conference & General & 1 \\
8 & International Conference on the Foundations of Software Engineering (FSE) & Conference & SWE & 1 \\
9 & International Journal of Frontiers in Engineering Technology & Journal & General & 1 \\
10 & International Symposium on Mixed and Augmented Reality & Conference & XR & 1 \\
11 & International Symposium on Software Reliability Engineering (ISSRE) & Symposium & SWE & 1 \\
12 & International Workshop on Quality and Measurement of Software Model-Driven Development & Workshop & SWE & 1 \\
13 & International Workshop on Artificial Intelligence in Software Testing & Workshop & SWE & 1 \\
14 & International Conference on Software Engineering (ICSE) & Tool & SWE & 1 \\
15 & International Workshop on Security for XR and XR for Security & Workshop & XR + SP & 1 \\
16 & Journal of Interactive Media (i-com) & Journal & HCI & 1 \\
17 & Jurnal Buana Informatika (JBI) & Journal & General & 1 \\
18 & Pacific Rim International Symposium on Dependable Computing (PRDC) & Conference & General & 1 \\
19 & Research Challenges in Information Science (RCIS) & Conference & General & 1 \\
20 & International Conference on Virtual Worlds and Games for Serious Applications (VS-Games) & Conference & XR & 1 \\
21 & International Conference on Reliability, Maintainability and Safety (ICRMS) & Conference & General & 1 \\
22 & ACM Transactions on Computer-Human Interaction & Journal & HCI & 1 \\
23 & IEEE Annual International Symposium Virtual Reality & Conference & XR & 1 \\
24 & ACM Transactions on Privacy and Security & Journal & SP & 1 \\
% 25 & Annual ACM Symposium on User Interface Software and Technology & Symposium & HCI & 1 \\
25 & Annual Ubiquitous Computing, Electronics \& Mobile Communication Conference (UEMCON) & Conference & General & 1 \\
26 & Applied Sciences & Journal & General & 1 \\
27 & Assembly Automation & Journal & General & 1 \\
28 & Conference on Graphics, Patterns and Images & Conference & XR & 1 \\
29 & HCI International (HCII) & Conference & HCI & 1 \\
30 & IEEE Transactions on Services Computing & Journal & General & 1 \\
31 & International Conference on Multimedia Information Processing and Retrieval (MIPR) & Conference & General & 1 \\
32 & IEEE Transactions on Visualization and Computer Graphics & Journal & CG & 1 \\
33 & Immersive Projection Technology Workshop & Workshop & XR & 1 \\
34 & International Conference on Actual Problems of Electronic Instrument Engineering (APEIE) & Conference & General & 1 \\
35 & International Conference on Computer Science and Electronics Engineering & Conference & General & 1 \\
36 & International Conference on Emerging Trends \& Innovation in ICT (ICEI) & Conference & General & 1 \\
37 & International Conference on Information and Communication Technology Convergence (ICTC) & Conference & General & 1 \\
38 & International Conference on Metaverse Computing, Networking and Applications (MetaCom) & Conference & XR & 1 \\
39 & The Computer Journal & Journal & General & 1 \\
\hline
\end{longtblr}

\restoregeometry
